# Supplementary material for: Reaching Full Correlation through Nonorthogonal Configuration Interaction: A Second-Order Perturbative Approach
Source: arXiv:2005.03962 ancillary file (2020-07-29)
Supplement: Supplementary file 1 [file supporting_information.pdf]

# Reaching Full Correlation through Nonorthogonal Configuration Interaction: A Second-Order Perturbative Approach — Supporting Information

Hugh G. A. Burton[1, a)] and Alex J. W. Thom[1, b)]
*Department of Chemistry, University of Cambridge, Lensfield Road, Cambridge, CB2 1EW, U.K.*

(Dated: 28 July 2020)

## SI. HOLOMORPHIC HARTREE–FOCK STATES OF LITHIUM FLOURIDE

The holomorphic Hartree–Fock[1–3] (h-HF) states of LiF (6-31G) used to define the NOCI basis in the main text have an intriguing pattern of interconnectivity. Here we provide a detailed discussion on the nature of these states to demonstrate how they are related through Coulson–Fischer points[4] along the potential energy surface. To illustrate these features, we compare the complex-valued h-HF energy of each state, defined as[2]

$$E_{\text{h-HF}} = \frac{\langle \Phi^* | \hat{H} | \Phi \rangle}{\langle \Phi^* | \Phi \rangle}, \tag{1}$$

and the conventional real energy given by the expectation value

$$E_{\text{HF}} = \frac{\langle \Phi | \hat{H} | \Phi \rangle}{\langle \Phi | \Phi \rangle}. \tag{2}$$

Note that a complex-valued h-HF state will not be a stationary point of the conventional real HF energy.[3] Since all real HF states are also stationary points of the h-HF energy, only states with complex-valued orbital coefficients are referred to as h-HF solutions.

In the main text, we identified a total of nine low-lying h-HF stationary states that had a significant contribution to the NOCI wave function. These states correspond to the ionic RHF ground state (A), a low-lying doubly-degenerate neutral UHF state

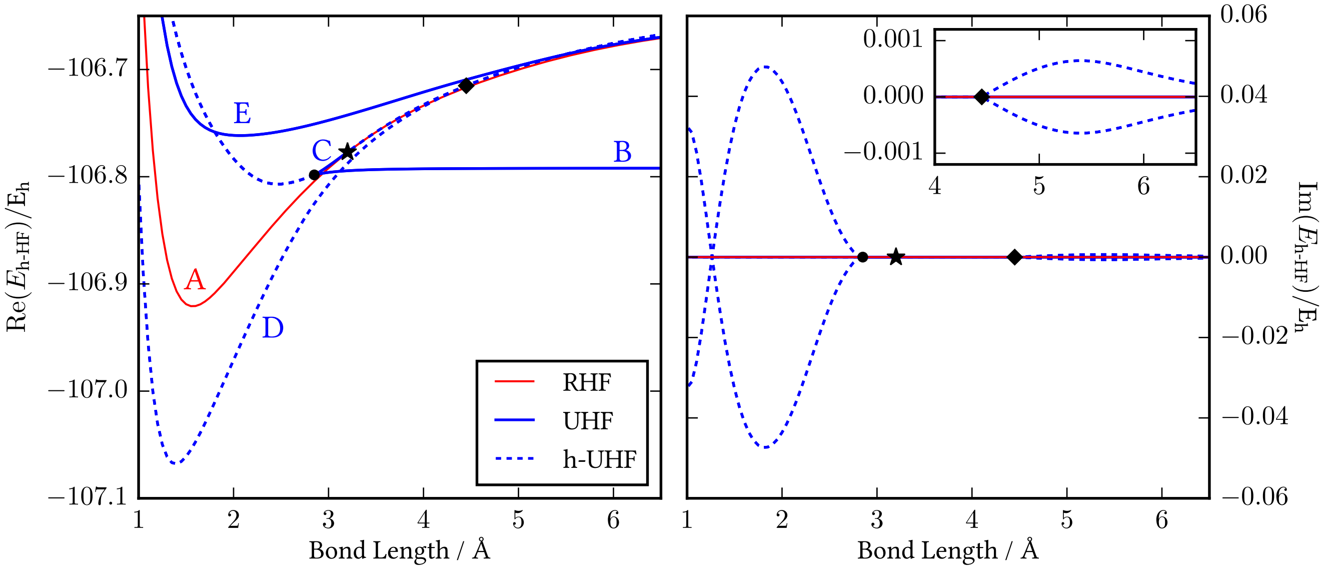


FIG. 1: Real (left) and imaginary (right) components of the h-HF energy (1) for the nine h-HF states identified in LiF (6-31G). The Coulson–Fischer points where states coalesce are indicated by black symbols. *Dot:* the real C and B states coalesce at two degenerate "pair-annihilation" points. *Star:* the real C states coalesce with the ionic A state at a "confluence" point. *Diamond:* the complex-valued C states coalesce with the complex-valued D states at two Coulson–Fischer points in the complex-plane, after which both pairs of states continue with complex h-HF energies related by complex conjugation.

---

a)Electronic mail: hb407@cam.ac.uk
b)Electronic mail: ajwt3@cam.ac.uk

(B) which coalesces with a third doubly-degenerate UHF state (C) at around 2.8 Å, a doubly degenerate h-UHF state (D) with complex-valued coefficients across all geometries, and a high-energy doubly-degenerate UHF state (E) that is real across all geometries. Since Eq. (1) is complex-valued in general, the real (left panel) and imaginary (right panel) components of the h-HF energy for these states are shown in Fig. 1. All complex-valued h-HF states appear in complex-conjugate pairs that become strictly degenerate if their h-HF energy is real.[3,5]

The C state displays the most interesting behaviour and is involved in three Coulson–Fischer points along the binding curve. At a bond length of 3.0 Å, this h-HF solution corresponds to a real HF state where one electron occupies a delocalised bonding orbital split between the Li and F atoms. As the bond length shortens, the C state eventually coalesces with the neutral B state at two doubly-degenerate Coulson–Fischer points that correspond to "pair-annihilation" points (black dot).[3] Beyond this Coulson–Fischer point, both the C and B states continue with complex-valued orbital coefficients and h-HF energies, with the states in each pair related by complex-conjugation. Notably, at around 1.25 Å, these pairs appear to become instantaneously degenerate when the imaginary component of their h-HF energies vanishes, although they do not coalesce at this point. In contrast, moving away from 3.0 Å towards larger bond lengths, we find that the real C states first coalesce with the ionic A state at a three-fold "confluence" point (black star),[3] before extending as h-UHF states with purely real h-HF energies. Moving further towards the dissociation limit, these complex-valued C states eventually coalesce with the complex-valued D states at two doubly-degenerate Coulson–Fischer points (black diamond) in the complex plane. Beyond this Coulson–Fischer point, both pairs of states again extend with complex-valued energies related by complex conjugation. As a result, we find that the C state is involved in *all* coalescence points between the states identified in LiF.

Although the D state has complex-valued orbital coefficients across all geometries, we find that its h-HF energy is purely real for bond lengths shorter than the Coulson–Fischer point at 4.4 Å, where it coalesces with the C state. While the h-HF approach is inherently non-Hermitian,[3] we have recently demonstrated that a h-HF wave function which is symmetric with respect to the combined parity-inversion $\mathcal{P}$ and time-reversal $\mathcal{T}$ operator (referred to as $\mathcal{PT}$-symmetry) must have strictly real h-HF energies.[5] While there is no centre of inversion in LiF, and thus the wave function cannot be $\mathcal{PT}$-symmetric, it is possible to extend the $\mathcal{PT}$-symmetry argument to show that a h-HF wave function with only $\mathcal{T}$-symmetry will also have a strictly real h-HF energy.[6] Pure $\mathcal{T}$-symmetry in a h-UHF wave function corresponds to the case where the spin-up and spin-down molecular orbitals are related by complex conjugation. As expected, we find that the D state conserves this $\mathcal{T}$-symmetry for all bond lengths shorter that than the Coulson–Fischer point at 4.4 Å and thus has a strictly real h-HF energy. Although these h-HF energies are real, they are not required to be variational[3] and hence the D state has a h-HF energy that falls below the true HF ground state in the equilibrium region.

Finally, to understand the significance of each h-HF state in the NOCI expansion, we consider their real energies defined by the expectation value (2), as shown in Fig. 2. Firstly, when considering the conventional energies, the coalescence of the C state with the A and D states becomes clearer as the bond is stretch towards dissociation (black diamond). Furthermore, although the D state has the lowest real component of the h-HF energy in the equilibrium, its conventional HF energy is actually the

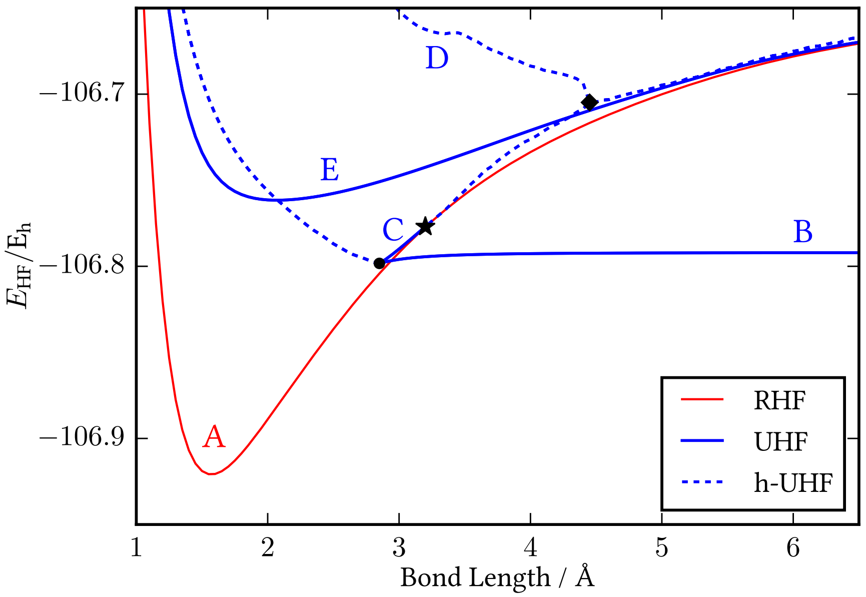


FIG. 2: Conventional HF energy (2) for the nine h-HF states in LiF, with the position of Coulson–Fischer points indicated by a black dot. The ionic RHF (A) and neutral UHF (B) states provide the HF ground-state energy and cross at around 3.0 Å.

highest out of all the states considered and it does not provide a major contribution to the low-lying NOCI states. In fact, the conventional energies demonstrate that the major contributors to the NOCI ground state are the RHF and UHF ground states representing the ionic and neutral configurations respectively, leading to the adiabatic NOCI energies identified in the main text.

## REFERENCES

[1]Hiscock, H. G.; Thom, A. J. W. Holomorphic Hartree–Fock Theory and Configuration Interaction. *J. Chem. Theory Comput.* **2014**, *10*, 4795.
[2]Burton, H. G. A.; Thom, A. J. W. Holomorphic Hartree–Fock Theory: An Inherently Multireference Approach. *J. Chem. Theory Comput.* **2016**, *12*, 167.
[3]Burton, H. G. A.; Gross, M.; Thom, A. J. W. Holomorphic Hartree–Fock Theory: The Nature of Two-Electron Problems. *J. Chem. Theory Comput.* **2018**, *14*, 607.
[4]Coulson, C. A.; Fischer, I. XXXIV. Notes on the molecular orbital treatment of the hydrogen molecule. *Philos. Mag.* **1949**, *40*, 386.
[5]Burton, H. G. A.; Thom, A. J. W.; Loos, P.-F. Parity-Time Symmetry in Hartree–Fock Theory. *J. Chem. Theory Comput.* **2019**, *15*, 4374.
[6]Burton, H. G. A. Holomorphic Hartree–Fock Theory: Moving Beyond the Coulson–Fischer Point. Ph.D. thesis, University of Cambridge, U.K., 2020.
